# Supplementary material for: Establishing CP Violation in $b$-Baryon Decays
Source: arXiv:2409.02821 source file (2025-06-05)
Supplement: Supplementary file 1 [file appendix.tex]

\appendix
\section{Topology classification}\label{sec:topo}
Resort to topological diagram classification, with all strong interactions included, the $\Lambda_b\to p\mathcal{M}_{\bar{u}d},p\mathcal{M}_{\bar{u}s}$ decays have the following topological diagrams fig.~\ref{fig:topo}. There are four tree level topological diagrams: $T$, the color-allowed external W-emission diagram; $C^\prime$, the color-commensurate W-emission diagram; $E_2$, the W-exchange diagram with the meson formed by the quark decayed from light quark; $B$, the bow-tie W-exchange diagram with the meson formed by the light spectator quark. There are six penguin level topological diagrams contributing to the $\Lambda_b\to p\mathcal{M}_{\bar{u}d},p\mathcal{M}_{\bar{u}s}$ decays: $P^C$, $P^{C^\prime}$, $P^{E_1^u}$, $P^B$, $P^{E_1^d}$ and $P^{E_2}$.
\begin{figure*}[htbp]
	\centering
	\subfigure{
		\begin{minipage}[]{0.22\linewidth}
			\includegraphics[width=1.7in]{figures/topoT.png}
		\end{minipage}
	}
	\subfigure{
		\begin{minipage}[]{0.22\linewidth}
			\includegraphics[width=1.7in]{figures/topoC2.png}
		\end{minipage}
	}
	\subfigure{
		\begin{minipage}[]{0.22\linewidth}
			\includegraphics[width=1.7in]{figures/topoE2.png}
		\end{minipage}
	}
	\subfigure{
		\begin{minipage}[]{0.22\linewidth}
			\includegraphics[width=1.7in]{figures/topoB.png}
		\end{minipage}
	}
	
	\subfigure{
		\begin{minipage}[]{0.22\linewidth}
			\includegraphics[width=1.7in]{figures/topoPC1.png}
		\end{minipage}
	}
	\subfigure{
		\begin{minipage}[]{0.22\linewidth}
			\includegraphics[width=1.7in]{figures/topoPC2.png}
		\end{minipage}
	}
	\subfigure{
		\begin{minipage}[]{0.22\linewidth}
			\includegraphics[width=1.7in]{figures/topoPE1u.png}
		\end{minipage}
	}
	\subfigure{
		\begin{minipage}[]{0.22\linewidth}
			\includegraphics[width=1.7in]{figures/topoPB.png}
		\end{minipage}
	}
	
	\subfigure{
		\begin{minipage}[]{0.22\linewidth}
			\includegraphics[width=1.7in]{figures/topoPE1d.png}
		\end{minipage}
	}
	\subfigure{
		\begin{minipage}[]{0.22\linewidth}
			\includegraphics[width=1.7in]{figures/topoPE2.png}
		\end{minipage}
	}
	\caption{Topological diagrams contributing to $\Lambda_b\to p\mathcal{M}_{\bar{u}d},p\mathcal{M}_{\bar{u}s}$ decays.}
	\label{fig:topo}
\end{figure*}

\begin{figure}[t]
	\includegraphics[scale=0.5]{figures/feyn-Cprime.png}
	\caption{A typical diagram for the $\Lambda_b\to p\pi^-$ decay, where two hard-gluon exchanges are necessary for forming the energetic final state. This diagram dominates the contribution to the $P^{C^\prime}$ topology.}
	\label{fig:feyn-Cprime}
\end{figure}

\begin{table*}
    \centering
    
    \begin{tabular*}{165mm}{c@{\extracolsep{\fill}}cccc|cccc}
		\hline
		\hline
        $\Lambda_b\to p\pi^-$ & $|S|$ & $\phi(S)^\circ$ & Real($S$) & Imag($S$) & $|P|$ & $\phi(P)^\circ$ & Real($P$) & Imag($P$)\\
		\hline
        $P^{C_1}_f$ &    30.55 &     0.00 &    30.55 &     0.00 &    43.05 &     0.00 &    43.05 &     0.00\\
        $P^{C_1}_{nf}$ &     2.27 &   -98.47 &    -0.33 &    -2.25 &    12.30 &  -100.05 &    -2.15 &   -12.12\\
        $P^{C_2}$ &     1.12 &   177.72 &    -1.12 &     0.04 &     1.75 &  -155.88 &    -1.59 &    -0.71\\
        $P^{E_1^u}$ &     2.22 &  -152.81 &    -1.97 &    -1.01 &     3.32 &   114.21 &    -1.36 &     3.02\\
        $P^B$ &     0.29 &   112.90 &    -0.11 &     0.27 &     0.36 &  -108.46 &    -0.11 &    -0.34\\
        $P^{E_1^d}+P^{E_2}$ &     2.46 &   -93.85 &    -0.17 &    -2.46 &     1.60 &    86.42 &     0.10 &     1.60\\
        O3 and O4 &    27.39 &   -11.38 &    26.85 &    -5.41 &    38.89 &   -12.69 &    37.94 &    -8.55\\
        \hline
        $P^{C_1}_f$ &    29.12 &     0.00 &    29.12 &     0.00 &    39.73 &   180.00 &   -39.73 &     0.00\\
        $P^{C_1}_{nf}$ &     0.66 &   121.56 &    -0.35 &     0.57 &     1.05 &   -74.21 &     0.28 &    -1.01\\
        $P^{C_2}$ &    13.42 &  -110.09 &    -4.61 &   -12.60 &    14.78 &    66.76 &     5.83 &    13.58\\
        $P^{E_1^u}$ &     7.97 &   -80.18 &     1.36 &    -7.85 &     6.39 &   113.89 &    -2.59 &     5.84\\
        $P^B$ &     1.58 &   -41.70 &     1.18 &    -1.05 &     1.26 &   176.31 &    -1.26 &     0.08\\
        $P^{E_1^d}+P^{E_2}$ &     1.66 &  -106.50 &    -0.47 &    -1.59 &     1.97 &   -26.79 &     1.76 &    -0.89\\
        O5 and O6 &    34.58 &   -40.65 &    26.23 &   -22.53 &    39.81 &   153.75 &   -35.71 &    17.61\\
		\hline
		\hline
    \end{tabular*}
    \caption{Penguin contributions $O_3\sim O_6$ for the $\Lambda_b\to p\pi^-$ decay.}
    \label{tab:pi-O3-O6}
\end{table*}

\begin{table*}
    \centering
    
    \begin{tabular*}{165mm}{c@{\extracolsep{\fill}}cccc|cccc}
		\hline
		\hline
        $\Lambda_b\to pK^-$ & $|S|$ & $\phi(S)^\circ$ & Real($S$) & Imag($S$) & $|P|$ & $\phi(P)^\circ$ & Real($P$) & Imag($P$)\\
		\hline
        $P^{C_1}_f$ &    37.28 &     0.00 &    37.28 &     0.00 &    53.00 &     0.00 &    53.00 &     0.00\\
        $P^{C_1}_{nf}$ &     2.81 &   -87.44 &     0.13 &    -2.81 &    15.64 &   -99.55 &    -2.60 &   -15.43\\
        $P^{E_1^u}$ &     2.97 &  -151.13 &    -2.60 &    -1.44 &     4.47 &   111.57 &    -1.64 &     4.16\\
        $P^{E_1^d}$ &     3.01 &   -92.29 &    -0.12 &    -3.01 &     2.07 &    87.07 &     0.11 &     2.07\\
        O3 and O4 &    35.43 &   -11.82 &    34.68 &    -7.25 &    49.72 &   -10.66 &    48.86 &    -9.20\\
		\hline
        $P^{C_1}_f$ &    40.85 &     0.00 &    40.85 &     0.00 &    55.60 &   180.00 &   -55.60 &     0.00\\
        $P^{C_1}_{nf}$ &     1.15 &   106.44 &    -0.33 &     1.10 &     1.60 &   -75.51 &     0.40 &    -1.55\\
        $P^{E_1^u}$ &    10.45 &   -75.46 &     2.62 &   -10.11 &     8.48 &   111.13 &    -3.06 &     7.91\\
        $P^{E_1^d}$ &     4.09 &  -108.15 &    -1.28 &    -3.89 &     1.23 &     5.62 &     1.22 &     0.12\\
        O5 and O6 &    43.81 &   -17.12 &    41.87 &   -12.90 &    57.40 &   173.53 &   -57.03 &     6.47\\
		\hline
		\hline
    \end{tabular*}
    \caption{Penguin contributions $O_3\sim O_6$ for the $\Lambda_b\to pK^-$ decay.}
    \label{tab:K-O3-O6}
\end{table*}
